# Supplementary material for: Differentiable Robot Rendering
Source: arXiv:2410.13851 source file (2024-10-17)
Supplement: Supplementary file 1 [file supp.tex]

include canonical gaussian renderings
